# Supplementary material for: CRT-6D: Fast 6D Object Pose Estimation with Cascaded Refinement Transformers
Source: arXiv:2210.11718 source file (2022-10-21)
Supplement: Supplementary file 1 [file supplementary.tex]

\section{Supplementary}
\label{sec:Supplementary}

\onecolumn
\begin{table}[]
\resizebox{\linewidth}{!}{%
\begin{tabular}{c|c|cc|cccc|cccc}
\Xhline{5\arrayrulewidth}
Method                    & PVNet       & \multicolumn{2}{c|}{DeepIM} & \multicolumn{4}{c|}{GDR-Net}                                           & \multicolumn{4}{c}{Ours}                                               \\ \hline
N.S.O.                    & 1           & \multicolumn{2}{c|}{21}     & \multicolumn{2}{c|}{1}                       & \multicolumn{2}{c|}{21} & 21        & \multicolumn{1}{c|}{21}          & 21        & 21          \\ \hline
Metric                    & AUC ADD(-S) & AUC ADD-S   & AUC ADD(-S)   & AUC ADD-S & \multicolumn{1}{c|}{AUC ADD(-S)} & AUC ADD-S & AUC ADD(-S) & AUC ADD-S & \multicolumn{1}{c|}{AUC ADD(-S)} & AUC ADD-S & AUC ADD(-S) \\ \Xhline{3\arrayrulewidth}
002\_master\_chef\_can    & 81.6        & 93.1        & 71.2          & 96.6      & \multicolumn{1}{c|}{71.1}        & 96.3      & 65.2        &           & \multicolumn{1}{c|}{}            & 98.38     & 79.47       \\ \hline
003\_cracker\_box         & 80.5        & 91.0        & 83.6          & 84.9      & \multicolumn{1}{c|}{63.5}        & 97.0      & 88.8        &           & \multicolumn{1}{c|}{}            & 86.18     & 57.21       \\ \hline
004\_sugar\_box           & 84.9        & 96.2        & 94.1          & 98.3      & \multicolumn{1}{c|}{93.2}        & 98.9      & 95.0        &           & \multicolumn{1}{c|}{}            & 99.68     & 97.58       \\ \hline
0005\_tomato\_soup\_can   & 78.2        & 92.4        & 86.1          & 96.1      & \multicolumn{1}{c|}{88.9}        & 96.5      & 91.9        &           & \multicolumn{1}{c|}{}            & 95.77     & 92.53       \\ \hline
006\_mustard\_bottle      & 88.3        & 95.1        & 91.5          & 99.5      & \multicolumn{1}{c|}{93.8}        & 100.0     & 92.8        &           & \multicolumn{1}{c|}{}            & 99.10     & 93.89       \\ \hline
007\_tuna\_fish\_can      & 62.2        & 96.1        & 87.7          & 95.1      & \multicolumn{1}{c|}{85.1}        & 99.4      & 94.2        &           & \multicolumn{1}{c|}{}            & 99.30     & 93.84       \\ \hline
008\_pudding\_box         & 85.2        & 90.7        & 82.7          & 94.8      & \multicolumn{1}{c|}{86.5}        & 64.6      & 44.7        &           & \multicolumn{1}{c|}{}            & 97.00     & 92.10       \\ \hline
009\_gelatin\_box         & 88.7        & 94.3        & 91.9          & 95.3      & \multicolumn{1}{c|}{88.5}        & 97.1      & 92.5        &           & \multicolumn{1}{c|}{}            & 99.95     & 97.99       \\ \hline
010\_potted\_meat\_can    & 65.1        & 86.4        & 76.2          & 82.9      & \multicolumn{1}{c|}{72.9}        & 86.0      & 80.2        &           & \multicolumn{1}{c|}{}            & 88.47     & 80.27       \\ \hline
011\_banana               & 51.8        & 91.3        & 81.2          & 96.0      & \multicolumn{1}{c|}{85.2}        & 96.3      & 85.8        &           & \multicolumn{1}{c|}{}            & 97.68     & 91.21       \\ \hline
019\_pitcher\_base        & 91.2        & 94.66       & 90.1          & 98.8      & \multicolumn{1}{c|}{94.3}        & 99.9      & 98.5        &           & \multicolumn{1}{c|}{}            & 99.82     & 97.35       \\ \hline
021\_bleach\_cleanser     & 74.8        & 90.3        & 81.2          & 94.4      & \multicolumn{1}{c|}{80.5}        & 94.2      & 84.3        &           & \multicolumn{1}{c|}{}            & 95.54     & 81.53       \\ \hline
024\_bowl*                & 89.0        & 81.4        & 81.4          & 84.0      & \multicolumn{1}{c|}{84..0}       & 85.7      & 85.7        &           & \multicolumn{1}{c|}{}            & 89.29     & 89.29       \\ \hline
025\_mug                  & 81.5        & 91.3        & 81.4          & 96.9      & \multicolumn{1}{c|}{87.6}        & 99.6      & 94.0        &           & \multicolumn{1}{c|}{}            & 99.98     & 92.53       \\ \hline
035\_power\_drill         & 83.4        & 92.3        & 85.5          & 91.9      & \multicolumn{1}{c|}{78.7}        & 97.5      & 90.1        &           & \multicolumn{1}{c|}{}            & 99.19     & 94.07       \\ \hline
036\_wood\_block*         & 71.5        & 81.9        & 81.9          & 77.3      & \multicolumn{1}{c|}{77.3}        & 82.5      & 82.5        &           & \multicolumn{1}{c|}{}            & 93.10     & 93.10       \\ \hline
037\_scissors             & 54.8        & 75.4        & 60.9          & 68.4      & \multicolumn{1}{c|}{43.7}        & 63.8      & 49.5        &           & \multicolumn{1}{c|}{}            & 67.51     & 35.63       \\ \hline
040\_larger\_marker       & 35.8        & 86.2        & 75.6          & 87.4      & \multicolumn{1}{c|}{76.2}        & 88.0      & 76.1        &           & \multicolumn{1}{c|}{}            & 98.16     & 89.41       \\ \hline
051\_large\_clamp*        & 66.3        & 74.3        & 74.3          & 69.3      & \multicolumn{1}{c|}{69.3}        & 89.3      & 89.3        &           & \multicolumn{1}{c|}{}            & 93.70     & 93.70       \\ \hline
052\_extra\_large\_clamp* & 53.9        & 73.3        & 73.3          & 73.6      & \multicolumn{1}{c|}{73.6}        & 93.5      & 93.5        &           & \multicolumn{1}{c|}{}            & 93.02     & 93.02       \\ \hline
061\_foam\_brick*         & 80.6        & 81.9        & 81.9          & 90.4      & \multicolumn{1}{c|}{90.4}        & 96.9      & 96.9        &           & \multicolumn{1}{c|}{}            & 96.04     & 96.04       \\
\Xhline{3\arrayrulewidth}
Average                   & 73.4        & 88.1        & 81.9          & 89.1      & \multicolumn{1}{c|}{80.2}        & 91.6      & 84.3        &           & \multicolumn{1}{c|}{}            & 95.68     &      88.05   \\ \hline
FPS                       &             &             &               &           & \multicolumn{1}{c|}{}            &           &             &           & \multicolumn{1}{c|}{}            &           &           \\
\Xhline{5\arrayrulewidth}
\end{tabular}
}
\end{table}
